# Supplementary material for: Transient contacts between filaments impart its elasticity to branched actin
Source: arXiv:2409.00549 ancillary file (2024-09-09)
Supplement: Supplementary file 1 [file SupplementaryMaterials.pdf]

# Transient contacts between filaments bestow its elasticity to branched actin

—

# Supplementary Text

Bouzid *et al.*

Here we present the detailed reasoning and procedures underlying the discussion of the main text. Sec. S1 presents the rationale for the central role of interfilament contacts in branched networks by showing that an ideal tree-like structure is critically coordinated, implying that its elastic moduli in the absence of contacts should vanish in the thermodynamic limit. It also presents the data extraction procedure used to generate Fig. 2(b). Sec. S2 and S3 then respectively describe our experimental and numerical procedures. Finally, Sec. S4 details our theoretical model.

## S1 Fundamentals of branched network rigidity

To give a rigorous foundation to the argument of Fig. 1(A) of the main text and understand the origin of the elasticity of branched networks, here we discuss their rigidity in the absence of any interfilament contact and considering only intrafilament interactions. We show that such networks are infinitely compliant in the thermodynamic limit. This is consistent with the absence of a linear elastic modulus in our experiments and simulations, and highlights the crucial role of contacts in stiffening the network under further compression. This stands in contrast with the well-defined linear elasticity of crosslinked networks.

To facilitate our discussion as well as numerical simulations, here and in Sec. S3 we model actin filaments as a collection of discrete elastic elements. This description is equivalent to a standard worm-like-chain model in the limit of small elements. We thus regard branched networks as a collection of $N$ interacting discrete vertices in $d$ dimensions. The interactions between the vertices dictate a set of optimal distances and angles between them [Fig. S1(a)], and it is useful to study the extent to which it is possible to deform the network without violating any of these optimality conditions. In this view, pioneered by Maxwell a century and a half ago [1], interactions are assimilated to constraints whose number must equal or exceed the number of internal degrees of freedom of the network ($2N-3$ for $d=2$ or $3N-6$ for $d=3$) to prevent the presence of soft modes of network deformation. In a more complete framework [2], one notes that redundant constraints on a subset of points can however enable additional soft modes in other parts of the network. We however need not consider these so-called states of self-stress here, as none are present in the structures discussed in this section.

In the absence of any states of self-stress, the rigidity of our networks is controlled by their relative number of internal degrees of freedom and constraints. Here we show by recursion that these numbers are always equal. The first step of the recursion is shown on the left of Fig. S1(b): the simplest possible branched network, composed of two vertices and one joining segment, has $2\times 3=6$ degrees of freedom in $d=3$ dimensions. Among those, 5 are global degrees of freedom (three translations and two rotations), leaving 1 internal degree of freedom. The system additionally has one constraint of the "bond extension" type. As a result this networks has as many constraints as internal degrees of

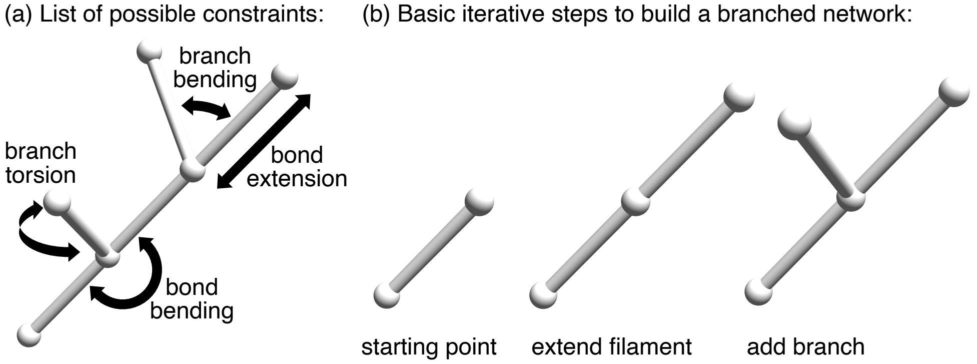


Figure S1: Branched networks are critically coordinated, implying their modulus vanishes in the thermodynamic limit in the absence of interfilament contacts. (a) Branched network model based on discrete elements. Each sphere represents a discrete vertex. Molecular interactions within the filaments favor a uniform equilibrium distance and alignment between vertices belonging to the same filament, while Arp2/3 branches must form a $\simeq 70°$ angle with their mother filament. In our constraint counting argument, all network deformations represented by black arrows on the figure are penalized energetically. Thus each of them is associated with one constraint. (b) The two elementary steps involved in the construction of a branched network: filament elongation and addition of a branching points. All branched networks considered here can be built by applying these steps iteratively.

freedom. It thus sits exactly at the isostatic point, namely the transition between the undercoordinated and the overcoordinated regime. Adding an additional vertex to this network, as further shown in the middle panel of Fig. S1(b), adds three degrees of freedom but also three constraints: one “bond extension” constraint and two “bond bending” angular constraints associated to the bending of the filament in each of the two directions orthogonal to its main axis. Such an addition thus keeps the network isostatic. Another possible addition is that of a branching point, which we show on the right-hand panel of Fig. S1(b). There, the number of degrees of freedom is again increased by three while additional constraints are also introduced. In the case represented here, namely that of the first branch in the system, there are two such constraints: one of the “bond extension” type, and one of the “branch bending” type. As the network is no longer axially symmetric, it moreover acquires one last global degree of freedom. This takes the total number of degrees of freedom of the systems to 12, including 6 global degrees of freedom. The remaining 6 internal degrees of freedom are stabilized by 3 “bond extension” constraints, two “bond bending” constraints and one “branch bending” constraints. In the case of subsequent branch additions, the initial network is already axially asymmetric, implying that the number of global degrees of freedom remains equal to 6. In that case however, the addition of the branch brings three new constraints: one “bond extension” constraint, one “branch bending” constraint and one “branch torsion” constraint. Note that the relevance of this last angular constraint in branched actin network has not been directly characterized to our knowledge.

A branched network deprived of its “branch torsion” constraints would not be critically coordinated (isostatic), but instead undercoordinated (hypostatic). Within the framework developed in the main text and in Sec. S4, this undercoordination would be described by a distance to isostaticity $n = 1$. In that sense, our inclusion of branch torsion constraints in the discussion of the previous paragraph constitutes a conservative assessment of the coordination of the network. In addition, the introduction of possible filament breaks in the ideal branched network considered here would also lower the coordination of the network.

As any branched network topology can be generated through a sequence of the two steps outlined in Fig. S1(b), and since both of these steps preserve the critical coordination of the network, we conclude that the simple branched networks considered here are exactly isostatic. Such networks are also sometimes characterized as being at their so-called bending critical point. As discussed in

Refs. [3, 4], networks endowed with this critical coordination have a vanishingly small linear elastic modulus in the thermodynamic limit. In addition, they exhibit diverging non-affine displacements. This means that the branches forming a large branched network should undergo large, uncoordinated motions when the network is compressed. Now reintroducing the possibility of contacts between neighboring branches that we have ignored until now, we realize that such large displacements must induce collisions between branches, and therefore result in the formation of contacts, which rigidify the network as discussed in the main text. Therefore, while the undercoordinated character of branched networks abolishes their linear response, it also results in their immediate nonlinear stiffening through the formation of contacts.

### Extraction procedure for the fiber packing data from the literature

We obtain all the non-actin data in Fig. 2(B) of the main text by extracting data from the literature. The original references cited in the main text all report data on the compression of fiber packings, either under the form of stress-strain stress-volume relationships. From these data points, we extract the differential modulus numerically by taking the stress-strain derivative. We then plot this differential modulus as a function of stress.

## S2 Experimental Materials & Methods

**Magnetic pincher.** Our experimental approach relies on a new technique that we recently developed named the Magnetic Pincher. The magnetic pincher aims to accurately measure the mechanical properties of submicron to micron sized structures using the magnetic attraction between superparamagnetic microparticles. When placed in a uniform magnetic field, such microparticles attract each other in the direction of the field while they repel in the orthogonal direction. As a result, they self-organize into pairs or chains aligned with the field direction. Two consecutive microparticles within a pair or chain thus exert a dipolar attraction on one another. We use this dipolar force to induce a controlled deformation in an object of interest interposed between the two microparticles. We accurately calculate the stress applied by the microparticles on the object based on the magnitude of the magnetic field, the distance between the microparticles, their dimensions and their magnetic susceptibility. The deformation of the object of interest is not directly measured using fluorescence but through the displacement of the magnetic microparticle that we obtain with a precision of a few nanometers. This technique can be implemented using either commercially available microbeads (Dynabeads, which are highly monodisperse in diameter) [5] or superparamagnetic microcylinders fabricated in the laboratory as in the present work [6]. We describe the cylinder fabrication protocol briefly below, and in detail in Ref. [7].

**In vitro reconstitution of Arp2/3 actin networks.** We reconstitute Arp2/3 actin network growth *in vitro* using well-established methods. We first graft a nucleation promoting factor on the surface of a micron-sized magnetic microcylinder, and subsequently put it in presence of a cocktail of monomeric actin, Arp2/3, capping protein, profilin and, when specified [Fig. 2(B) of the main text], cofilin. The mix of actin, Arp2/3 and the proteins listed above allow the regulation of actin polymerization and the formation of dense actin branched networks by known biochemical mechanisms [8, 9]. The role of the nucleation promoting factor is to activate the Arp2/3 complex. We specifically use the pWA C-terminal domain of the human actin nucleation-promoting factor WAS protein or WASP (P42768) as a nucleation factor. This WASP-pWA protein contains WH2 and proline-rich domains that promote actin polymerization by Arp2/3 activation, actin-profilin interaction and actin desequestration [10].

We used Plasmid pGEX4T1-GST-pWA-His coding for a fusion WASP-pWA (residues 150-502) protein containing a N-terminal GST and C-terminal polyHis tag to transform E. Coli Rosetta™

2(DE3) competent cells (Novagen, 71400-3). We expressed the the fusion WASP-pWA through IPTG induction with 0.5 mM IPTG and incubation for another 3h. We pelleted and washed the bacteria in pH 7.4 binding buffer with 20 mM Tris, 200 mM NaCl, 45 mM Imidazole, 0.1% NP40 and 1 mM beta-mercaptoethanol, containing Complete™ protease inhibitor EDTA-free (Roche, 11873580001). We resuspended the bacterial pellets in $1/50^{th}$ of the original culture volume and lyzed them using a cell disruptor (One shot model, Constant System Inc.). We purified the proteins by affinity chromatography using a HisTrap HP affinity column (Cytiva). We stored the samples aliquoted at −80°C.

Actin, Arp2/3, capping protein, profilin and cofilin are kindly provided by Guillaume Romet-Lemonne and Antoine Jégou's team in Institut Jacques Monod. WASP-pWA has been purified by Cesar Valencia-Gallardo. We used the following concentrations: 6 $\mu$M actin, 95 nM Arp2/3, 90 nM capping protein and 30 $\mu$M profilin in a buffer with 6 mM Hepes, 1.8 mM ATP, 6.2 mM DTT, 140 $\mu$M Dabco, 80 mM KCl, 100 $\mu$M $CaCl_2$ and 6 mM $MgCl_2$ at pH 7.8. Experiments with cofilin used the same concentrations except 500 nM cofilin, 4 $\mu$M actin, and 12 $\mu$M profilin.

**Cylinder fabrication and functionalization.** Our fabrication of magnetic cylinders follows the protocol of Tavacoli *et al.* [7]. In brief, we fabricate an array of wells out of polydimethylsiloxane (PDMS) using standard soft lithography techniques. We fill the polydimethylsiloxane (PDMS) molds with a mixture of 300-nm superparamagnetic colloids (50% w/w, purchased from Ademtech), ethoxylated trimethylolpropanetriacrylate (ETPTA) monomer and a thermoinitiator. As a result of curing at 130°C for 2 hours the small colloids become embedded in a solid polymeric matrix. The resulting microcylinders have a radius of 3 $\mu$m and a length comprised between 12 and 18 $\mu$m as imposed by the mold. Microcylinders are subsequently functionalized with GST-pWA while still in the PDMS mold to ensure that only the upper face is activated for branched actin network growth. The subsequent extraction is performed in a solution of 1 mg/mL Bovine Serum Albumine (BSA) in PBS to passivate the other faces of the microcylinders. To facilitate the extraction, the PDMS mold is bent and introduced into a small tube containing the BSA solution. The tube is subjected to sonication during 10-30 seconds. The geometry of the tube forces the mold to bend in its larger dimension, while bending in the thinner dimension is obtained by pushing on the opposite face of the mold with a rigid rod. Great care is needed at this stage to preserve WASP-pWA activity.

**Experimental setup.** The experimental setup is based on an Zeiss Axio A1 inverted microscope with a 100X/1.4 NA oil immersion Apochromat. The stage of the microscope is modified to hold two magnetic coils with a soft iron core. These coils generate a uniform magnetic field in the chamber with a magnitude that can be varied externally from 0 to 80 mT using a bipolar operational power supply (Kepco, New York City, NY, USA) to feed the coil with up to 5 A electrical current. This maximum current corresponds to an 80 mT homogenous magnetic field in the chamber. The field magnitude as well as image acquisition are controlled by a lab-made Labview (National Instruments, Austin, TX, USA) program. The camera is an ORCA Flash 4.0 CMOS camera (Hamamatsu).

**Force and distance analysis.** The distance between two neighbouring cylinders corresponds to the thickness of the actin network. Its value is calculated on every image by a sub-pixel correlation of two regions of interest drawn inside each cylinder with an estimated error on the displacement of around 2.5 nm [6]. The network thickness is measured on the first image of the video with an error estimated to 63 nm [11]. The force $F$ applied between two cylinders depends on the cylinder dimensions, their distance, their magnetic susceptibility (measured on each new batch of cylinders) and the magnetic field magnitude. We estimate it by interpolating a series of finite elements analyses as described previously [6].

**Mechanical measurements.** To access the mechanical response of the actin networks, we vary the magnetic field from 3 to 60 mT and then back in 2 s. The time dependence of the magnetic field is quadratic, implying that the force depends roughly linearly on time. The attractive force $F$ between cylinders depends on the inter-cylinder distance, and is thus larger for thinner networks. We compute the stress as the ratio of the force $F$ to the surface $S$ of the cylinder face. We compute the true strain as $\gamma = \ln(H_0/H)$ from the thicknesses $H_0$ and $H$ of the network immediately prior to and during compression. We derive strain-stress from these measurements during compression. The tangent elastic modulus reported in Figs. 3(B) and 4(B) of the main text is the local slope of these stress-strain curves. We compute it for stress values regularly spaced on a logarithmic scale to emphasize the response at low stress. To obtain the stress-volume curves of Figs. 2(C), 3(A) and 4(A) of the main text, we compute the network volume as $V = H \times S$ (likewise $V_0 = H_0 \times S$). We verify through fluorescence imaging that the lateral enlargement of the actin network during compression is negligible.

**Experimental averaging.** To obtain an average stress volume curve, we first record the minimum values $V_m$ of the volume reached by each network. These correspond to conditions of maximal stress. For a series of networks which all have a different $V_m$, we compute the average value of the stress corresponding to the same value of $(V_0/V)^3$ up to the smallest $(V_0/V_m)^3$ in this series. This prevents us from computing average stresses for values of $(V_0/V)^3$ that are only reached by a some of our networks. Indeed, such a sample would be biased towards the mechanical response of softer networks. To explore a large range of $(V_0/V)^3$, the aforementioned series of networks do not include all the networks we probe experimentally. Instead, we cull our data by removing the softest and the stiffest networks from our analysis. To this end, we first sort the curves in ascending order of $(V_0/V_m)^3$ and exclude the first (stiffest) quartile of curves. To mitigate the resulting bias, we also remove the last (softest) quartile. We use such culled series of networks to compute the average stress and tangent elastic moduli. The error bars on all graphs in the main text materialize the standard error.

# S3 Numerical simulations

Our numerical simulations of branched networks consist in two successive steps. In Sec. S3.1, we detail the first, where we generate the topology and initial geometry of model contact-free, unfrustrated networks with or without crosslinkers. This geometrical structure is then endowed with mechanical properties in Sec. S3.2, where we introduce intra-filament extensional (*i.e.*, stretching) and bending elasticity, as well as a procedure to introduce a controlled amount of entanglements in initially contact-free structures.

## S3.1 Procedure to generate contact-free branched networks

Consistent with the known mechanisms of branched actin polymerization, our network generation procedure proceeds through the stochastic addition of branching points at the top surface of the network, resulting in an anisotropic network of approximately uniform density (Sec. S3.1.1) to which crosslinkers can be added. In the resulting model network, all intra-filament bonds are at their equilibrium length, all angular constraints are satisfied and filaments do not touch, implying that the network is initially in an unstressed, contact-less elastic ground state (Sec. S3.1.2). We additionally develop a mean-field description of our growth algorithm which predicts its volume fraction as a function of the filament branching rate (Sec. S3.1.3).

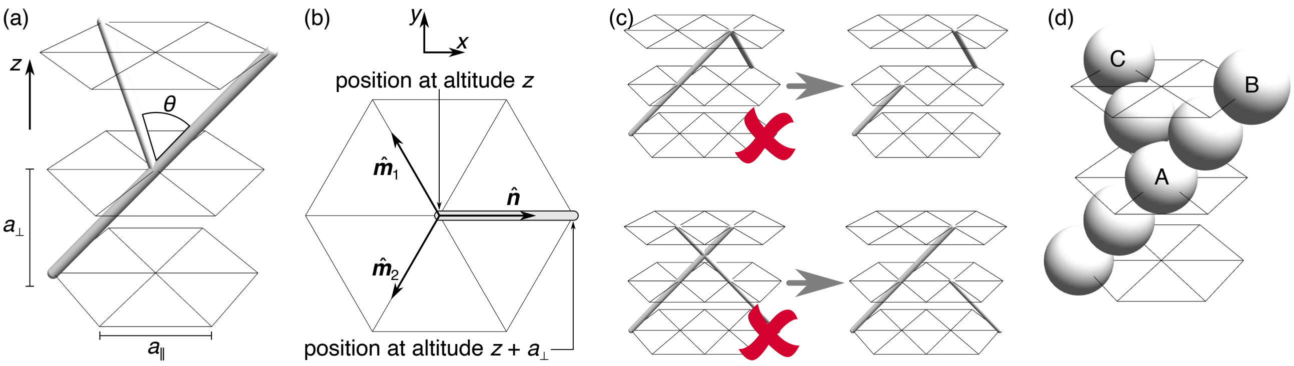


Figure S2: Layered growth model for the filament structure. (a) Side view of the stacked triangular lattices and of a branching event, with the branching angle $\theta$ indicated. (b) Top view of the triangular lattice, with the direction $\hat{\mathbf{n}}$ of the main filament and the two possible branching directions $\hat{\mathbf{m}}_1$ and $\hat{\mathbf{m}}_2$ indicated. Note that either branching direction $\hat{\mathbf{m}}_1$ and $\hat{\mathbf{m}}_2$ gives the same branching angle $\theta$ in three dimensions. (c) Illustration of the two types of potential overlap situations that our algorithm avoids (left) and of one of the two equally likely filament termination events that it enforces to prevent each one (right). (d) Position of the repulsive spheres used in the mechanical simulations to implement the inter-filament impenetrability for the configuration shown in panel (b). Consecutive spheres along a filament (but not across a branching point) overlap slightly.

### S3.1.1 Network topology

The initial structure of our branched network is based on a three-dimensional lattice formed by stacking two-dimensional lattices in the direction of network growth, which we denote by $z$ [Fig. S2(a)]. The $z = 0$ layer of the lattice represents the initial state of the network as its growth begins: each site of the triangular lattice (whose lattice spacing we denote by $a_\parallel$) is either empty or occupied by a filament, and each filament points in one of the six directions of the lattice. As growth proceeds, additional layers are added sequentially to the network with a vertical spacing $a_\perp$. All filaments in the bottom layer grow at the same speed and make the same angle with the vertical direction $z$. A filament that intersects a layer with altitude $z$ at a position $\mathbf{x}$ while pointing in direction $\hat{\mathbf{n}}$ comprised within the $(x, y)$ plane thus intersects the next plane at position $\mathbf{x} + a_\parallel\hat{\mathbf{n}} + a_\perp\hat{\mathbf{z}}$. The values of $a_\parallel$ and $a_\perp$ are discussed in the next section.

In addition to this deterministic growth process, when moving from the first to the second layer each filament branches with a probability $b \in [0, 1]$. When a filament branches, the algorithm picks either one of the two orientations $\hat{\mathbf{m}}_i$ indicated in Fig. S2(b) with equal probability, and adds a filament at position $\mathbf{x} + a_\parallel\hat{\mathbf{m}}_i + a_\perp\hat{\mathbf{z}}$ that points in direction $\hat{\mathbf{m}}_i$, *i.e.*, away from the branching site.

In a physical branched actin network, the proliferation of filaments due to the branching process is compensated by the random capping of the growing filament barbed ends. This capping is more frequent in a dense network, as it tends to move the WASP-pWA-coated microcylinders apart faster, which leaves straggling filaments more vulnerable to capping. To model this filament density homeostasis, we impose that a site of our lattice cannot be simultaneously occupied by two filaments. To enforce this condition, in cases where several filaments are headed for the same lattice site we terminate all but one of them, which we choose at random. In addition, if two neighboring triangular lattice sites attempt to each send a filament towards the other, then one of the two filaments is terminated at random [Fig. S2(c)]. While this mechanism is more local than the global balance described above, it has the advantage of ensuring that filaments do not overlap in the initial state of the network.

We generate the full network by iterating this layer stacking process as many times as needed. The structure of the network depends on our initial choice of number of filaments in the $z = 0$ layer up to an altitude $\approx a_\perp/b$, where the balance between filament branching and capping becomes established. To avoid artifacts linked to this transient regime we systematically delete the bottom layers formed

by our growth algorithm and use only network structures well into the stationary regime.

In addition to establishing the structure of branching points throughout our network, this procedure allows up to add crosslinkers to mimick experiments using $\alpha$-actinin. We add such crosslinkers by randomly bonding neighboring sites within a network layer with a bond with rest length $a_{\parallel}$.

#### S3.1.2 Network geometry

In the numerical simulations described below (Sec. S3.2), the vertices of our network are the center of spherical particles which repel one another when in contact, ensuring the filaments' impenetrability. We use the distance between two such lattice sites belonging to the same filament as our unit length. To ensure that undeformed filaments that are not connected do not form contacts in the absence of deformation, we place two such particles between triangular lattice sites belonging to the same filament as shown in Fig. S2(d). The equilibrium distance between the centers of two such particles is therefore equal to 1/2 in our simulations units. Following this choice, we select the lattice spacings $a_{\parallel}$ and $a_{\perp}$ to satisfy two constraints. First, the length of segment $AB$ must be equal to 1. Second, the angle $\theta = \widehat{CAB}$ must be equal to the branching angle, namely 70°. These constraints impose

$$a_{\parallel} = \sqrt{\frac{1 + 2\cos\theta}{3}} \simeq 0.749231 \tag{S1a}$$

$$a_{\perp} = \sqrt{\frac{2 - 2\cos\theta}{3}} \simeq 0.662309. \tag{S1b}$$

#### S3.1.3 Filament volume fraction

To predict the fraction of the volume occupied by the filaments, we devise a mean-field model whereby the probability that any site is occupied at altitude $z$ is denoted by $p_z$ and considered constant across all sites. If a site is occupied, it adopts each one of the six possible orientations with probability 1/6. Since every filament attempts to grow to the next layer (although this attempt may be thwarted by our termination mechanism), it attempts to grow its main filament towards each of its neighboring sites with probability $p_z/6$, and a secondary branch with probability $bp_z/6$. As a result, the probability with which a site at altitude $z + a_{\perp}$ is targeted by each of its neighbors is $(1 + b)p_z/6$.

We now use this result to compute the probability $1 - p_{z+a_{\perp}}$ with which a site at altitude $z + a_{\perp}$ is *un*occupied within the mean-field approximation. This will be the case if any of the following four mutually exclusive circumstances is realized:

- None of the six neighboring sites at altitude $z$ has targeted the site of interest with a filament. Probability of occurrence:
$$P_1(b, p_z) = \left(1 - \frac{1+b}{6} p_z\right)^6 . \tag{S2}$$
- The following independent (in the mean-field approximation) events all occur:
  - The site of interest is occupied at altitude $z$ (probability $p_z$)
  - The site neighboring the site of interest in direction $\hat{\mathbf{n}}$ targets the site of interest (probability $(1 + b)p_z/6$)
  - The site of interest prevails in the resulting termination contest (probability 1/2)
  - No other neighboring site targets the site of interest (probability $[1 - (1 + b)p_z/6]^5$)

  Overall probability of occurrence:
$$P_2(b, p_z) = \frac{1+b}{12} p_z^2 \left(1 - \frac{1+b}{6} p_z\right)^5 . \tag{S3}$$

- The following independent events all occur:
  - The site of interest is occupied (probability $p_z$)
  - The site of interest launches a branch in the direction $\hat{\mathbf{m}}_i$ with $i = 1$ or 2 (probability $b$).
  - The site neighboring the site of interest in direction $\hat{\mathbf{m}}_i$ targets the site of interest (probability $(1 + b)p_z/6$)
  - The site of interest prevails in the resulting termination contest (probability 1/2)
  - No other neighboring site targets the site of interest (probability $[1 - (1 + b)p_z/6]^5$)

  Overall probability of occurrence:

$$P_3(b, p_z) = \frac{(1+b)b}{12} p_z^2 \left(1 - \frac{1+b}{6} p_z\right)^5 . \tag{S4}$$

- The following independent events all occur:
  - The site of interest is occupied (probability $p_z$)
  - The site of interest launches a branch in the direction $\hat{\mathbf{m}}_i$ with $i = 1$ or 2 (probability $b$).
  - The site neighboring the site of interest in direction $\hat{\mathbf{n}}$ targets the site of interest (probability $(1 + b)p_z/6$)
  - The site neighboring the site of interest in direction $\hat{\mathbf{m}}_i$ targets the site of interest (probability $[1 + b)p_z/6)$
  - The site of interest prevails in both resulting capping contests (probability 1/4)
  - No other neighboring site targets the site of interest (probability $[1 - (1 + b)p_z/6]^4$)

  Overall probability of occurrence:

$$P_4(b, p_z) = \frac{(1+b)^2 b}{144} p_z^3 \left(1 - \frac{1+b}{6} p_z\right)^4 . \tag{S5}$$

The occupancy probability within the mean-field assumption is thus given by the recursion:

$$p_{z+a_\perp} = 1 - [P_1(b, p_z) + P_2(b, p_z) + P_3(b, p_z) + P_4(b, p_z)] \tag{S6}$$

After a transient regime, this recursion converges to a unique, stable stationary solution which we numerically determine by setting $p_{z+a_\perp} = p_z = p^*(b)$ in Fig. S3. Furthermore, if $b$ is small then $p^*(b) \approx b$ and the transient regime has a duration of order $b^{-1}$. The recursion can then be approximated by a continuum equation in the $p_z \approx b \ll 1$ regime, yielding to lowest order in $b$:

$$a_\perp \partial_z p = b p_z - \frac{p_z^2}{2}, \tag{S7}$$

which yields a typical relaxation length $a_\perp/b$ and an asymptotic probability

$$p^*(b) \underset{b \to 0}{\sim} 2b, \tag{S8}$$

in very good agreement with both simulations and the exact fixed point of the mean-field equation up to $b \simeq 0.1$ (Fig. S3).

To compute the volume fraction occupied by the network at low $b$, we neglect the volume of the filament ends and branching points and assimilate the filament to a cylinder of length $bN_s$ and radius 1/4, where $N_s$ denotes the total number of lattice sites in the system. The volume per lattice site is $a_\perp a_\parallel^2 \frac{\sqrt{3}}{2}$, implying a filament volume fraction

$$\phi = \frac{3\pi}{4\sqrt{2}} \frac{b}{(1 + 2\cos\theta)\sqrt{1 - \cos\theta}} \simeq 1.21966 \times b. \tag{S9}$$

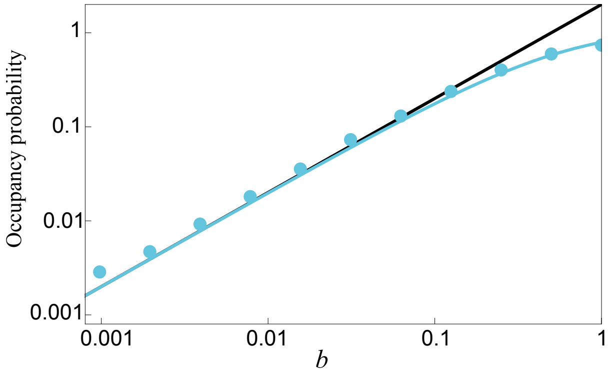


Figure S3: Occupancy probability $p^*(b)$ of a lattice site in our growth model. The circles shows the result of the full simulated procedure, the blue line shows the numerically calculated fixed point of Eq. (S6) and the black line shows the asymptotic result Eq. (S8).

## S3.2 Elasticity simulations

Our coarse-grained molecular dynamics simulations capture the mechanical response of branched actin networks using minimal, generic ingredients. We introduce physical interactions between network constituents in Sec. S3.2.1. Section S3.2.2 then describes the protocol we use to strain these networks. Section S3.2.3 presents our protocol to compute the resulting stresses. Section S3.2.4 discusses the procedure we use to generate pre-entangled networks to model branched actin grown under stress. Section S3.2.5 describes our method for counting contacts in the simulation.

### S3.2.1 Interactions in our coarse-grained numerical model

We translate the structures generated in Sec. S3.1 as a 3D system of discrete chains of spherical monomers Fig. S4(a) with center-to-center spacing 1/4. These monomers are not meant to literally represent individual actin monomers, and should be understood as a coarse-grained version thereof. They interact through a potential energy composed of three terms:

$$\mathcal{U}(\mathbf{r_1},...,\mathbf{r_N}) = \sum_{\substack{i<j \\ \text{bonded pairs}}} \mathcal{U}_{\text{intra-chains}}(r_{ij}) + \sum_{\substack{i<j \\ \text{non bonded}}} \mathcal{U}_{\text{inter-chains}}(r_{ij}) + \sum_{\substack{i<j<k \\ \text{bonded triplets}}} \mathcal{U}_{\text{bending}}(\mathbf{r}_i, \mathbf{r}_j, \mathbf{r}_k)\,. \tag{S10}$$

Here $\mathbf{r}_i$ denotes the position vector of the $i$-th monomer in the filament and where $r_{ij} = |\mathbf{r}_i - \mathbf{r}_j|$. Equation S10 is known to represent the Kremer and Grest bead springs model [12, 13]

The first contribution to Eq. (S10) accounts for a bonded interactions between monomers belonging to the same chain, given by a harmonic potential:

$$\mathcal{U}_{\text{intra-chains}}(r) = \frac{K}{2}\left(r - \frac{1}{2}\right)^2, \tag{S11}$$

which reflects the fact that the equilibrium bond length extension is equal to 1/2, and where $K$ is the (typically large) bonding elastic constant.

The second term is given by a repulsive potential meant to prevent the actin monomers from interpenetrating. We thus assimilate the individual vertices along a filament to repulsive spheres. We additionally assign a radius slightly large than half the equilibrium distance between vertices to the spheres in order to make sure that filaments cannot interpenetrate. We thus use a Weeks-Chandler-Andersen potential (WCA) [14] with range $2^{-5/6}$, implying

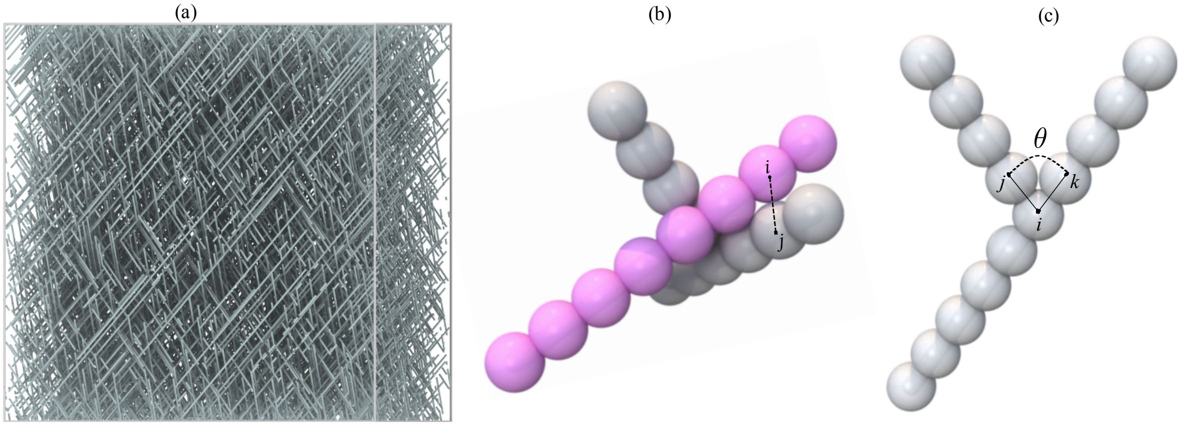


Figure S4: Illustration of our numerical simulations. (a) Typical contactless configuration showing only bonds between monomers (and not the monomers themselves). (b) Structure of a branching point. (c) Interaction between two monomers belonging to two different filaments.

$$\mathcal{U}_{\text{inter-chains}}(r) = \begin{cases} 4\epsilon\left[\left(\frac{1}{2r}\right)^{12} - \left(\frac{1}{2r}\right)^{6}\right] + \epsilon & \text{for } r \leq 2^{-5/6} \\ 0 & \text{for } r > 2^{-5/6} \end{cases} \tag{S12}$$

This term effectively enforces an excluded volume between filaments [Fig. S4(b)]. The energy $\epsilon$ denotes the strength of the repulsive interaction and both the potential energy and radial force vanish at the cutoff distance $r = 2^{-5/6}$.

The last term of the right-hand-side of Eq. (S10) is a three-body interaction that accounts for the bending rigidity of the filaments and acts on triplets of three consecutive bonded monomers $(j, i, k)$. It is given by:

$$\mathcal{U}_{\text{bending}}(\theta) = \frac{\kappa}{2}(\theta - \theta_0)^2, \tag{S13}$$

where $\theta = \arccos\left(\frac{\mathbf{r}_{ij}\cdot\mathbf{r}_{ik}}{|r_{ij}||r_{ik}|}\right)$. Denoting the filament diameter by $d$, the bending constant $\kappa$ is related to the persistence length through $\ell_p = \kappa d/k_BT$. This length however does not play a role in our simulations as we investigate the athermal limit of the networks' mechanics. The equilibrium angle $\theta_0$ is set equal to $\theta_0 = 180°$ for all triplets of consecutive monomers of the same filament. This guarantees straight filaments in the absence of stress. We use other values of $\theta_0$ at actin branching points, which are characterized by resting angles of 70°, 110° and 180° [Fig. S4(c)].

We assimilate the filament diameter to the distance between consecutive vertices along a simulated filament, *i.e.*, 1/2 in our length units. The quantity $\kappa$ plays the role of our unit of energy. In these units, we choose a filament bonding constant $K = 300$ and a repulsive energy $\epsilon = 1$, which ensure that the filaments are incompressible and impenetrable. When matching these units with the dimensional units in the main text, we set $\kappa = 4 \times 10^{-26}\,\text{J}\cdot\text{m}$ as is relevant for actin. We also fix the mesh size of our networks to the typical value observed in branched actin network, namely $\xi = d/\sqrt{b} = 40\,\text{nm}$. In practice we use a branching probability $b = 0.1$ throughout, which strikes a compromise between having realistically thin filaments (which requires monomers that are small compared to the mesh size) and fast simulations (which requires having comparatively few, large monomers). The network is characterized by its volume fraction $\phi \simeq 1.22b$ [see Eq. (S9)], and we use $N_m \simeq 4.10^4$ monomers in an initially cubic simulations box with linear size $\mathcal{L} \simeq 80d$.

### S3.2.2 Deformation protocol

To probe its elastic response, we subject the network to successive small incremental strain steps $\delta\gamma = \delta\mathcal{L}_z/\mathcal{L} = 0.01$ in the $z$ direction to mimic an uniaxial compression test [15]. More specifically, we first apply an instantaneous affine deformation $\Gamma_{\delta\gamma}$ to all monomers in the current configuration $\{\mathbf{r}_i\}$ such that the deformed configuration $\{\mathbf{r}'_i\}$ is given by

$$\mathbf{r}'_i = \Gamma_{\delta\gamma} \cdot \mathbf{r}_i = \begin{pmatrix} 1 & 0 & 0 \\ 0 & 1 & 0 \\ 0 & 0 & 1-\delta\gamma \end{pmatrix} \cdot \mathbf{r}_i \tag{S14}$$

The simulation box has periodic boundary conditions in the $x$ and $y$ direction and the top and bottom monomers of the gel are held in place. Upon compression of the gel, the top fixed monomers are translated downwards.

Following the affine deformation of Eq. (S14), the configuration $\{\mathbf{r}'_i\}$ is not at mechanical equilibrium, since the affine deformation does not give filaments a chance to bend to avoid the energetically costly compression. We therefore next let the system relax mechanically. To this end, we run a molecular dynamics simulation at constant box size and shape for a time interval $\tau$. Denoting by $\mathcal{T}_\tau$ the time evolution operator corresponding to this dynamics, we denote the new configuration of the system by

$$\mathbf{r}''_i = \mathcal{T}_\tau \mathbf{r}'_i, \tag{S15}$$

where $\mathcal{T}_\tau$ is derived from the damped equation of motion for each monomer:

$$m\frac{d^2\mathbf{r}_i}{dt^2} = \mathbf{F}^c_i + \mathbf{F}^f_i. \tag{S16}$$

Here $m$ is the mass of a monomer, $\mathbf{F}^c_i = -\nabla_{\mathbf{r}_i}\mathcal{U}$ is the conservative force derived from the potential of Eq. (S10) and $\mathbf{F}^f_i = -\eta d\mathbf{v}_i$ is the dissipative force associated with the coupling of the particle motion to an (implicit) surrounding fluid with viscosity $\eta/(6\pi)$. All simulations are performed for values of $m$ and $\eta$ in the slightly overdamped regime for optimal performance (the magnitude of the damping is immaterial to the final equilibrium state of the system). We use LAMMPS, an open-source molecular dynamics software package [16] where the equation of motion is solved using a Verlet algorithm with a time step $\delta t = 0.005\sqrt{(md^2/4\epsilon)}$.

After $n_c$ compression steps, the cumulative true strain is $\gamma = n_c\delta\gamma$ and the network configuration is

$$\mathbf{r}_{i,n} = (\mathcal{T}_\tau\Gamma_{\delta\gamma})^n\, \mathbf{r}_{i,0}\,, \tag{S17}$$

where $\{\mathbf{r}_{i,0}\}$ denotes the configuration of the starting structure. This procedure defines a finite rate of deformation $\dot\gamma = \delta\gamma/\tau$. We study the quasi-static limit for which $\dot\gamma \to 0$. More quantitatively, we define the natural time scale $\tau_0 = \eta d^3/\kappa$ associated with the microscopic dynamics, which corresponds to the time it takes a monomer subjected to a typical force of order $\kappa/d$ (or equivalently $\epsilon/d$ for our choice of parameters) to move over a distance equivalent to its diameter. We place ourselves in conditions where $\dot\gamma\tau_0 \sim 3.10^{-8}$, which we find guarantees that our results are insensitive to its specific value.

### S3.2.3 Stress calculation

The average state of stress of the network is given by the virial stress $\sigma_{\alpha\beta} = -\mathcal{L}^{-3}\sum_i \hat\sigma^i_{\alpha\beta}$, where the Greek subscripts stand for the Cartesian coordinates $(x, y, z)$. We recall that $\mathcal{L}$ is the linear size of simulation box and define $\hat\sigma^i_{\alpha\beta}$ as the contribution to the stress tensor of all the interactions involving

monomer $i$ [17]. We compute this quantity for each monomer by splitting the contributions of the two-body and the three-body forces according to

$$\hat{\sigma}^i_{\alpha\beta} = \sum_{n=1}^{N_2} r^i_\alpha F^{(2,n)i}_\beta + \sum_{n=1}^{N_3} r^i_\alpha F^{(3,n)i}_\beta. \tag{S18}$$

Here the first sum runs over all the $N_2$ pairs of interactions that involve the monomer $i$. The force $\mathbf{F}^{(2,n)i}$ is the force exerted on monomer $i$ specifically due to the $n$th two-body interaction. The second sum functions similarly for interacting triplets of particles. Since we consider only equilibrated systems, we disregard the kinetic contribution $-\mathcal{L}^{-3}\sum_i m_i \delta v^i_\alpha \delta v^i_\beta$ to the global stress tensor.

#### S3.2.4 Network pre-entanglement procedure

To mimic stressed growth in branched actin, we generate a controlled number of contacts through the following filament entanglement procedure:

1. We turn off the steric interactions given by Eq. (S12) for all monomers. This allows filaments to pass through each other.
2. We apply a predetermined affine compressive prestrain $\gamma_p = \delta\mathcal{L}_z/\mathcal{L}$ to the network [see Fig. 3(D-F) of the main text]. We use $\gamma_p \in [0.02, 0.2]$. Following the application of this prestress we let the system relax in the absence of steric interactions through a molecular dynamics simulation [Eq. (S16)]. During this process the filaments cross each other.
3. We slowly turn the steric interactions back on while still continuously letting the system evolve through molecular dynamics. This locks in the entanglements induced by the prestrain while avoiding the occurrence of large forces.
4. We apply an opposite prestrain $-\gamma_p$ to decompress the network and get it back to its the initial box size.
5. We again let the network relax through molecular dynamics to reach mechanical equilibrium. In this state the vertical component of the network stress vanishes.

As a result of the creation of filament entanglements during this procedure, our prestrained networks exhibit local density heterogeneities [Fig. S5(a-b)]. Additionally, the network typically does not relax back to its original size and ends up not filling the box. This effect is more pronounced for larger values of $\gamma_p$. To prevent the resulting low-density regions [Fig. S5(b)] from perturbing our characterization of the bulk properties of the network, we systematically delete these regions as well as the neighboring low-density network regions, which in practice correspond to a maximum thickness of $\simeq 3d$.

#### S3.2.5 Counting of the number of contacts

To compute the number of contacts per filament in the simulation as reported in the horizontal axis of Fig. 4 of the main text as well as Fig. S5(c), we first count the number of monomers that are within a distance $r_c = 2^{-5/6}$ (*i.e.*, within interacting distance) of at least one other monomer. We next reason that when two filaments contact, each filament contributes two monomers to the contact. That way the four contacting monomers form an interacting tetrahedron, which ensures the contact's mechanical stability. We thus divide the number of interacting monomers by two, divide the resulting number by the total number of filaments in the simulation and denote the resulting number as $\chi$.

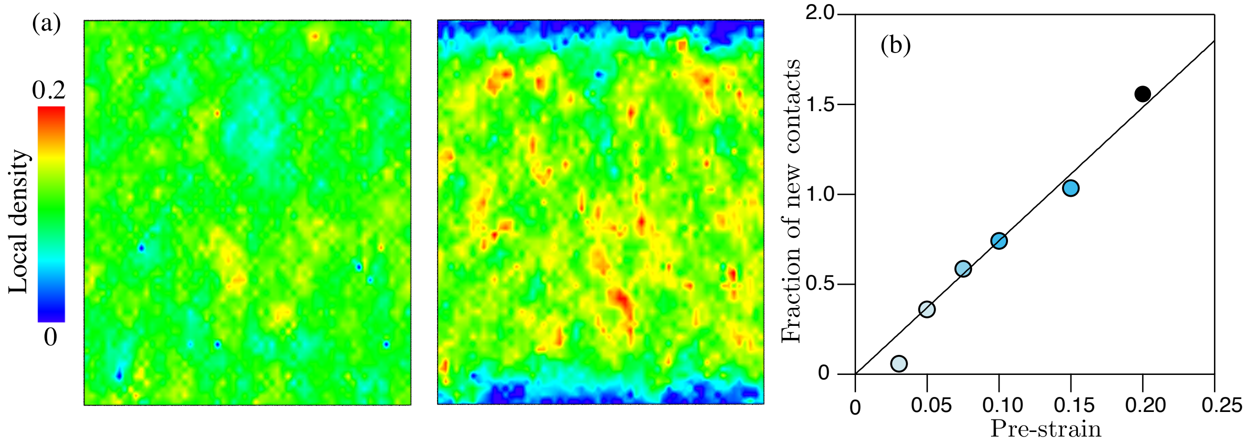


Figure S5: Characterization of our prestrained networks. (a) Prior to the imposition of prestress, the density of the network averaged in the $y$ direction and projected onto the $x, z$ plane is fairly homogeneous. Here the color scale represents the fraction of the box volume occupied by monomers. (b) Following the imposition of a prestrain $\gamma_p = 0.1$, the network displays strong heterogeneities due to newly formed entanglements. Note also the depleted (*blue*) regions at the top and bottom of the box, which outline the overall shrinkage of the network due to the procedure. (c) The fraction of newly created contacts is roughly linear in the imposed prestrain $\gamma_p$.

This number $\chi$ is however an unreliable estimate of the number of contacts per filament. Indeed, our simulations also include additional, spurious monomers that are in close proximity of one another but do not bring any new contacts to the network. This happens when contacting monomers merely reinforce additional preexisting constraints in the network, and typically occurs in the vicinity of its branching points. The number of such spurious contacts varies little over the course of the compression of a network. We thus assume that for each of our networks the number of spurious contacts is always equal to its value in the initial state of the network (*i.e.*, the state where the external stress vanishes, $\sigma = 0$). To estimate the number of contacts per filaments in this state, we thus rely on the initial number of contacts per filament $\alpha_0$ provided by the fits of Fig. 3 of the main text. We thus write the number of contacts per filament as

$$\alpha = \alpha_0 + (\chi - \chi_0), \tag{S19}$$

where $\chi_0$ is the number of productive + spurious contacts estimated in the network's initial state. We report the number $\alpha$ in the horizontal axis of Fig. 5 of the main text.

## S4 Analytical theory

Our theory for the elasticity of branched actin networks derives from ideas put forward by van Wyk in 1946 to describe the stiffening of another weakly coordinated filament system, namely sheep's wool, as its filaments form an increasing number of contacts under compression [18]. We present this original model in Sec. S4.1 under the form of a scaling argument, and obtain the corresponding pressure-volume relationship up to an integration constant. We additionally extend the model to derive the value of this constant in networks grown under an opposing compressive stress. While this approach is valid for networks with long filaments under relatively high compression, these conditions are not always fulfilled in our branched networks. In Sec. S4.2 we thus propose a more detailed model where weakly coordinated short filaments must be mechanically activated through the formation of contacts before they can participate in the network's elasticity (Fig. S6). We describe the implications of this mechanism for the network's pressure-volume relation in Sec. S4.3. We then apply this framework to networks grown under stress in Sec. S4.4. We extend our formalism to situations where crosslinkers

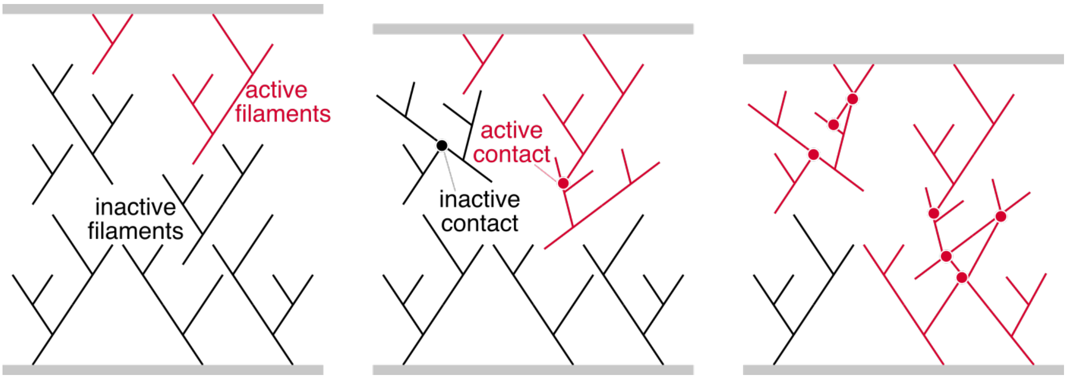


Figure S6: In a weakly coordinated branched network compressed between two plates, a pressure applied to the top plate initially (left panel) is felt only by a small fraction of active (red) filaments. By contrast, the inactive (black) filaments do not participate in the response to the outside pressure for lack of contacts with their neighbors. As the network is compressed (central panel), contacts form and some inactive filaments are turned into active ones. Upon sufficient compression (right panel), the active filaments percolate through the system and the network acquires a finite stiffness.

are present in Sec. S4.5. Finally, we analyze the values of the fitting parameters of the main text in view of our theoretical results in Sec. S4.6.

## S4.1 Scaling theory for a network with long branches

In the original van Wyk theory, a long filament of length $L$ (or several long filaments with total length $L$), diameter $d$ and bending modulus $\kappa$ is enclosed in a volume $V$. As the enclosure is compressed and the available volume is reduced, the initially loose filament randomly forms an increasing number of contacts with itself. This forces it to bend on smaller and smaller length scales, which can only be achieved at the cost of a rapidly increasing compressive stress.

To estimate the number of contacts the filament forms with itself, we subdivide it into $L/d$ "monomers" of length $d$. We estimate the contact probability between two monomers through the mean-field approximation that monomers are distributed within the enclosure in a uniform, uncorrelated fashion. The probability that a given monomer overlaps with another is thus of the order of the polymer volume fraction $\phi \approx Ld^2/V$, resulting in a total number of contacts

$$N_{\text{contacts}} \approx \phi L/d \approx L^2 d/V. \tag{S20}$$

As a result of these contacts, the filament is divided into a number of segments approximately equal to $N_{\text{contacts}}$. Each such segment has a characteristic length $\zeta = L/N_{\text{contacts}} \approx V/Ld$ [Fig. S7(a)]. In an enclosure of volume $V$ at equilibrium under a compressive stress $\sigma$, a typical segment is maintained in its (typically bent) shape by a force $f$. We now consider imposing a small additional strain $\mathrm{d}\gamma = \mathrm{d}V/V$ ($\mathrm{d}\gamma < 0$ for a compression) on the system, which requires increasing the stress $\sigma$ by a small $\mathrm{d}\sigma$. This additional compression is shared by all filaments within a horizontal cross-section of the network. Since the typical lateral spacing between two filaments is $\approx \sqrt{V/L}$, this corresponds to an increase of the load on an individual filament by $\mathrm{d}f \approx (V/L)\mathrm{d}\sigma$. Concomitantly, the additional strain $\mathrm{d}\gamma$ implies a relative motion of the ends of each filament segment by a distance

$$\mathrm{d}y \approx -\zeta \mathrm{d}\gamma = -\zeta \frac{\mathrm{d}V}{V}. \tag{S21}$$

We now consider the mechanics of a single bent filament segment, and note that moving its end by a

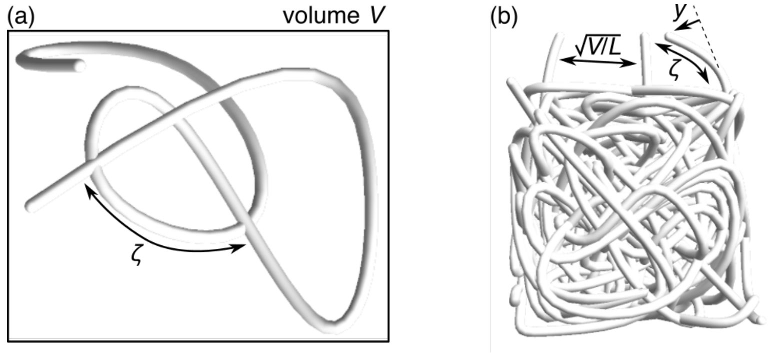


Figure S7: Our initial scaling argument relies on singling out the response of filament segments flanked by two contacts. (a) A filament confined in a volume $V$ randomly forms contacts with itself. The typical distance between consecutive contacts is $\zeta$. (b) As filaments grow, the deflection $y$ of a segment located at the growing surface of the network increases until it forms a contact with a neighboring filament, which is typically located at a distance $\sqrt{V/L}$. The typical segment length for which this happens fixes the value of $\zeta$ in the bulk.

length $\mathrm{d}y$ typically requires a force $\mathrm{d}f = (\kappa/\zeta^3)\mathrm{d}y$. This implies

$$\mathrm{d}\sigma \approx \frac{L}{V}\mathrm{d}f \approx \frac{L}{V}\frac{\kappa}{\zeta^3}\mathrm{d}y \qquad \Rightarrow \qquad \frac{\mathrm{d}\sigma}{\mathrm{d}V} = -\bar{\gamma}\frac{\kappa L^3 d^2}{V^4}, \tag{S22}$$

where $\bar{\gamma}$ is an undetermined numerical prefactor of order one. We integrate this relation over $V$ to find the pressure-volume relationship of the system:

$$\sigma = \frac{\bar{\gamma}\kappa L^3 d^2}{3V^3} - \sigma_\infty \tag{S23a}$$

$$= \sigma_\infty \left[\left(\frac{V_0}{V}\right)^3 - 1\right], \tag{S23b}$$

where the integration constant $\sigma_\infty = \bar{\gamma}\kappa L^3 d^2/3V_0^3$ is the absolute value of the stress required to expand the system to an infinite volume. Its value is directly related to $V_0$, the resting volume of the system. The relation Eq. (S23) is the main result of the original van Wyk theory [18], which does not tackle the question of predicting $\sigma_\infty$ from physical arguments. As shown in Fig. 2(B) of the main text, Eq. (S23) yields a good description of the strongly compressed cofilactin networks.

Equation (S23) additionally dictates the following stiffness-stress relation:

$$K = -V\frac{\mathrm{d}\sigma}{\mathrm{d}V} = 3(\sigma + \sigma_\infty). \tag{S24}$$

The presence of a power law scaling of $\sigma$ with $V$ in the $V \ll V_0$ limit as in Eq. (S23) is very robust. Variants of the van Wyk model where the distribution of the filaments is very anisotropic indeed still display it, albeit with a different power law [19]. These changes do not however affect the $K \underset{\sigma\gg\sigma_\infty}{\propto} \sigma$ scaling of Eq. (S24), which could help account for the collapse of the $K(\sigma)$ data shown in Fig. 2(A) of the main text across a wide range of different systems. Despite this success, in our branched networks this description breaks down in the low-compression ($\sigma \ll \sigma_\infty$) regime. There, the elastic plateau $K_0 = 3\sigma_\infty$ predicted by Eq. (S24) overestimates the stiffness of the networks. In the following subsections, we account for this discrepancy by taking into account the finite length of the network branches. As a rule of thumb, the infinite-filament-length approximation used in the present section is expected to fail when $\zeta$ is of the order of the branch length.

Our first approach to determining the dependence of the constant $\sigma_\infty$ on the network growth conditions assumes the simple case of growth under a large compressive stress $\sigma_g$. More specifically,

we assume that an outside wall imposes a stress $\sigma_g$ that is large enough that $\zeta$ is always smaller than the branch length. This stress deforms the network filaments during growth, leading to the formation of contacts. These contacts are subsequently locked into place as more filaments grow around them and filament entanglements proliferate. As a result, a substantial fraction of these contacts subsists even in the event where the compressive force is removed following the network growth phase, as shown in Fig. S5(b). The resting state of the network thus contains a finite density of contacts. To estimate this density, and thus $\sigma_\infty$, we count the number of contacts that form during growth. We focus our attention in the immediate neighborhood of the wall, where filament growth takes place as the Arp2/3 complex is activated and growing barbed ends are not yet capped. As an individual network filament grows, the opposing force from the wall tends to deform it. A long filaments is more easily deformed than a shorter one. As a result, a filament pushing against an opposing force becomes increasingly deflected as it grows longer, until the point where the deformation is so large that the filament runs into one of its neighbors [Fig. S7(b)]. When that happens, a contact between filaments form, which stabilizes the first filament and forms the mechanical foundation for the subsequent growth of the network. This scenario allows us to self-consistently derive an expression for the inter-contact length $\zeta$. Since the surface density of filaments is $L/V$, each growing filament is subjected to a force $f \approx V\sigma_g/L$ during growth. Under such a force, the lateral deflection $y$ of a filament of length $\zeta$ is of the order of $f\zeta^3/\kappa$. The contact with the neighboring filament occurs when the deflection $y$ is of the order of the lateral distance $\sqrt{V/L}$ between two filaments. This condition reads

$$\frac{V\sigma_g}{L}\frac{\zeta^3}{\kappa} = \sqrt{\frac{V}{L}}. \tag{S25}$$

By further using $\zeta \approx V/Ld$ as previously, we find

$$\zeta(\sigma_g) \approx \left(\frac{\kappa}{\sigma_g}\right)^{2/7} r^{-1/7} \tag{S26}$$

and thus

$$K_0 \approx \sigma_\infty \approx \frac{\kappa L^3 d^2}{V^4} \approx \frac{\kappa^{1/7}}{d^{4/7}}\sigma_g^{6/7}. \tag{S27}$$

This expression implies an almost linear dependence between the plateau modulus of the network and its growth pressure, consistent with the data of Fig. 3(C) of the main text. While the finite-filament-length corrections to Eqs. (S23) and Eq. (S24) discussed in Secs. S4.2 and S4.3 are quantitatively important in accounting for the data shown in Fig. 3 of the main text, the asymptotic reasoning leading to Eq. (S27) is actually a good approximation in practice, as further discussed in Sec. S4.4.

## S4.2 Mechanical activation of undercoordinated filaments

The theory described in Sec. S4.1 is well suited for networks whose filaments are each longer than the segment length $\zeta$. However, in cases where the filaments are short and the compression weak (implying a large $\zeta$), this regime may not be reached and the response of the network may deviate from Eq. (S23). Here we study such situations to account for the full mechanical responses presented in Figs. 3 and 4 of the main text.

The constraint counting argument presented in Sec. S1 finds that branched networks are exactly isostatic. As discussed there however, this constitutes a conservative assessment which may overestimate the number of constraints. It indeed disregards possible breaks in the experimental networks and assumes without direct evidence that the torsional rigidity of the Arp2/3 branching points is comparable with the actin bending stiffness (up to a multiplication by the segment length for dimensional reasons). In our simulations, this torsional rigidity actually vanishes. The branched networks

considered in the main text are thus likely to be hypostatic, *i.e.*, to have fewer constraints than degrees of freedom. To understand the qualitative implications of this hypostaticity, consider a single filament with fewer constraints than degrees of freedom. In the absence of the type of contacts discussed in Sec. S4.1, this filament can be moved without any elastic cost. According to Maxwell's argument [1], a network where such free filament motions are widespread can undergo large-scale deformations without changing its deformation energy and thus has a vanishing elastic modulus. When this network is significantly deformed however, contacts such as the ones discussed in the previous section proliferate and constrain the motion of the previously freely moving filament. The filaments then eventually become activated in the sense if Fig. S6, and the network stiffens.

Here we assess the proportion of activated filaments in a mean-field approximation. We thus disregard the intricacies of the network's branched geometry, and view it as a soup of hypostatic filaments of length $\ell$. In our terminology, a "filament" refers to a branch of the network, *i.e.*, the length of actin that starts with an Arp2/3 complex and terminates with a capping protein. We account for the connectivity due to the branched structure of the network in a simplified way by stating that each filament is missing $n \geq 0$ constraints to fully constrain its motion. The case $n = 0$ thus corresponds to the conservative constraint counting argument of Sec. S1: no missing constraints, exact isostaticity. In the case of our simulations, the missing torsional constraints and the fact that there is one torsional degree of freedom per filament in the thermodynamic limit suggest a value of $n$ close to one.

We denote by $p$ the probability that a specific filament is mechanically active and set out to determine the value of $p$ self-consistently. Following the reasoning leading to Eq. (S20), we find that the average number of contacts per filament is

$$\alpha = \bar{\alpha}\frac{N\ell^2 d}{V}, \tag{S28}$$

where $\bar{\alpha}$ is a geometrical prefactor of order one and $N$ is the total number of filaments present in the system. Not all contacts are equally effective at constraining the filament. If the filament comes in contact with an immobile, active filament, then the formation of the contact will have a mechanically stabilizing effect. This is the case of the "active contacts" of Fig. S6. Conversely, a contact with an inactive filament simply means that the two previously freely moving filaments must now move together, but this joint motion still does not cost any energy. This constitutes an "inactive contact". This implies that only active contacts contribute to filament stability. We thus introduce the average number $\beta = p\alpha$ of active contacts per filament. Because of fluctuations in filament length and network geometry, not all filaments have exactly $\beta$ active contacts. Instead, we assume that the number of active contacts per filament follows a Poisson distribution, namely

$$\mathcal{P}(k) = \text{Proba(filament of interest has } k \text{ active contacts)} = \frac{\beta^k}{k!}e^{-\beta}. \tag{S29}$$

This choice of distribution is equivalent to making the mean-field assumption that the probability per unit length of forming an active contact is constant along the length of the filaments. The probability that a filament is active can then be written as

$$p = \text{Proba(filament of interest has at least } n \text{ active contacts)} = \sum_{k=n}^{+\infty}\frac{\beta^k}{k!}e^{-\beta} = \lambda_n(\beta). \tag{S30}$$

Here we have defined

$$\lambda_n(\beta) = 1 - \frac{\Gamma(n,\beta)}{\Gamma(n)}, \tag{S31}$$

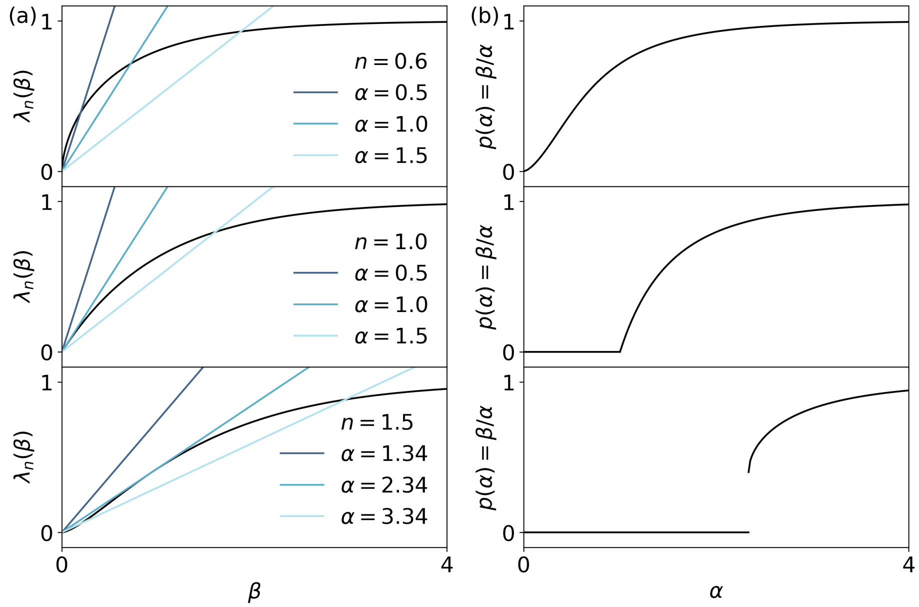


Figure S8: The activation of the network filaments proceeds through a mean-field percolation transition. (a) Illustration of the self-consistency condition of Eq. (S33). This condition gives the order parameter $\beta$ (number of activated contacts per filament) as a function of the control parameter $\alpha$. As discussed in the text, the nature of the transition depends on the value of $n$: the three subpanels illustrate the three possible cases $n < 1$, $n = 1$ and $n > 1$. The critical control parameters $\alpha^*$ for the three subpanels are 0, 1 and 2.34, respectively. (b) Filament activation probability as a function of $\alpha$ obtained by solving the self-consistency condition for the same values of $n$ as in (a). The three subplots respectively illustrate the three cases of a smoothly increasing $\beta$, a second-order transition and a first-order transition.

where $\Gamma(n, \beta)$ and $\Gamma(n)$ respectively denote the incomplete and complete gamma functions. The function $\lambda_n$ behaves as a power law for small $\beta$: $\lambda_n(\beta) \underset{\beta \to 0}{\sim} \beta^n / \Gamma(n+1)$. We additionally introduce

$$\mu_n(\beta) = \partial_\beta \lambda_n(\beta) = \frac{\beta^{n-1} e^{-\beta}}{\Gamma(n)}. \tag{S32}$$

In the following we use Eq. (S30) even for non-integer values of $n$ as a reasonable interpolation to describe systems where $n$ fluctuates locally, resulting in a non-integer average $n$.

Equation (S30) can be rewritten as

$$\frac{\beta}{\alpha} = \lambda_n(\beta), \tag{S33}$$

which serves as a self-consistency equation determining the value of $\beta$ and where $\alpha$ acts as a control parameter.

Equation (S33) can be interpreted graphically by realizing that its physically relevant solution is given by the rightmost intersection between the straight line and the $\lambda_n(\beta)$ curve in Fig. S8(a). In a weakly compressed system ($V$ large, thus $\alpha$ small) the straight line is very steep and the intersection occurs for a small value of $\beta$. Indeed, under such conditions, when two filaments come into contact the probability that one of them contacts further (activated) filaments is very low, and therefore both filaments remain inactive. As the volume of the system is decreased however, clusters of contacting filaments become more likely to percolate through the system, and the probability for an individual filament to be active approaches one as $\alpha$ increases to infinity. In this strong-compression regime, $\beta \gg 1$ and $\lambda_n(\beta) \simeq 1$ (or equivalently $p = 1$) as shown in Fig. S8(b). This implies $\beta = \alpha$ and recapitulates the regime discussed in Sec. S4.1.

The character of the transition between the weak- and strong-compression regimes depends on the value of $n$. For $n < 1$, the probability $p(\alpha)$ is strictly positive for all $\alpha > 0$ and there is no transition at finite $\alpha$. Conversely, for $n > 1$, this probability vanishes for $\alpha$ smaller than a critical value $\alpha^*(n)$. When $\alpha$ reaches $\alpha^*$, the system undergoes a first-order transition and $p$ jumps discontinuously to a finite value. In the marginal case $n = 1$, the transition is second order, and the problem has a simple closed-form analytical solution:

$$\beta(\alpha) = \alpha p(\alpha) = \begin{cases} 0 & \text{for } \alpha < 1 \\ \alpha + W_0\left(-\alpha e^{-\alpha}\right) & \text{for } \alpha \geq 1 \end{cases}, \tag{S34}$$

where $W_0$ is the principal branch of the Lambert W function. In the main text, we fit $n$ to both the experimental and numerical data and consistently find values of $n$ that are close to one. This suggests that Eq. (S34) provides an accurate and convenient way to determine $\beta$ in branched networks with finite length filaments.

### S4.3 Elastic response of an undercoordinated network

To assess the pressure-volume relationship of the undercoordinated branched networks described in Sec. S4.2, we apply a mechanical reasoning similar to that of Sec. S4.1.

Consider a single mechanically active filament. As in the discussion of Sec. S4.1, every contact in excess of isostaticity marks a boundary between two segments. An exactly isostatic filament with $k = n$ contacts thus consists of a single mechanically activated segment. Therefore filaments with $k \geq n$ have $k - n + 1$ segments, each with an average length of $\zeta(k) = \ell/(k - n + 1)$. As in Sec. S4.1, the typical spring constant associated with each segment is $\kappa/\zeta(k)^3$. Writing the specific area per filament as $V/L = V/(N\ell)$ and summing over the distribution of contact number $k$, we obtain a modified version of Eq. (S22):

$$\mathrm{d}\sigma = -\bar{\gamma}\frac{N\ell}{V}\sum_{k=n+1}^{+\infty}\mathcal{P}(k)\frac{\kappa}{\zeta(k)^3}\mathrm{d}y, \tag{S35}$$

where $\bar{\gamma}$ is again a dimensionless prefactor of order one. Here the sum runs only over filaments that have enough contacts to define at least two segments, as this is the minimum required for a filament to bend. Using Eqs. (S21), (S28) and (S29) we recast $\sigma$ as a function of the compression parameter $\alpha$ and obtain

$$\frac{\mathrm{d}\tilde{\sigma}}{\mathrm{d}\alpha} = g_n[\alpha p(\alpha)] = g_n(\beta), \tag{S36}$$

where we have defined the dimensionless compressive stress

$$\tilde{\sigma} = \frac{\bar{\alpha}}{\bar{\gamma}}\frac{\ell^3 d}{\kappa}\sigma \tag{S37}$$

and where the function $g_n$ is given by

$$g_n(\beta) = \sum_{k=n+1}^{+\infty}\frac{\beta^k}{k!}(k+1-n)^2 e^{-\beta} = \left[\beta^2 + (3-2n)\beta + (1-n)^2\right]\lambda_n(\beta) + \beta\left[\beta - \frac{(1-n)^2}{n}\right]\mu_n(\beta), \tag{S38}$$

which yields $g_n(\beta) \underset{\beta\longrightarrow 0}{\longrightarrow} 0$ for $n > 0$ and $g_n(\beta) \underset{\beta\to+\infty}{\longrightarrow} +\infty$. We use Eq. (S33) to compute the Jacobian of the change of variable $\alpha \to \beta$ as

$$J_n(\beta) = \frac{\mathrm{d}\alpha}{\mathrm{d}\beta} = \frac{1}{\lambda_n(\beta)}\left[1 - \frac{\beta\mu_n(\beta)}{\lambda_n(\beta)}\right] \tag{S39}$$

and use it to integrate Eq. (S36) into

$$\tilde{\sigma}(\beta) = \int_{\beta_0}^{\beta} g_n(b) J_n(b)\, \mathrm{d}b, \tag{S40}$$

where the integral has no simple analytic form in the general case but can be computed numerically. This implies the following definition for the function $S_n$ discussed in the main text [we recall that $\tilde{\sigma} = S_n(\alpha) - S_n(\alpha_0)$]:

$$S_n(\alpha) = \int_{\beta(\alpha^*)}^{\beta(\alpha)} g_n(b) J_n(b)\, \mathrm{d}b, \tag{S41}$$

where the function $\beta(\alpha)$ is defined as the solution of Eq. (S33), and where we define $\alpha^*(n) = 0$ for $n < 1$. The function $S_n(\alpha)$ does not have a closed-form expression in general, although one can be derived in the special case $n = 1$. The fits we perform in the main text indicate that $n$ is very close to 1 for our experimental and simulated networks, implying that $S_1(\alpha)$ describes these systems well. The explicit expression of $S_1(\alpha)$ is however cumbersome, and we therefore look for an approximation under the form of an easy-to-handle fraction of polynomials $S_1^{\text{approx}}(\alpha) = (\alpha-1)^3(a\alpha^2+b\alpha+c)/(\alpha^2+d\alpha+e)$. Here $a$ $b$, $c$, $d$ and $e$ are numerical coefficients to be determined. Remembering that $S_1(\alpha)$ is nonzero only on the interval $\alpha \in [1, \infty)$, we choose these coefficients to match the asymptotic behavior of $S_1(\alpha)$ in $\alpha \to 1^+$ and $\alpha \to +\infty$ respectively to third and second order, namely:

$$S_1(\alpha) = \frac{8}{3}(\alpha-1)^3 - \frac{7}{3}(\alpha-1)^4 + \frac{20}{9}(\alpha-1)^5 + o[(\alpha-1)^5] \tag{S42a}$$

$$S_1(\alpha) = \frac{\alpha^3}{3} + \frac{\alpha^2}{2} + o(\alpha^2). \tag{S42b}$$

This condition imposes 5 constraints on the coefficients of $S_1^{\text{approx}}(\alpha)$. The unique solution of this problem reads

$$S_1^{\text{approx}}(\alpha) \simeq \frac{(\alpha-1)^3}{3} \frac{14\alpha^2 + 149\alpha + 677}{14\alpha^2 + 86\alpha + 5}. \tag{S43}$$

In addition to closely matching the behavior of $S_1(\alpha)$ in $1^+$ and $+\infty$ by construction, we determine that the relative error committed by using $S_1^{\text{approx}}(\alpha)$ instead of $S_1(\alpha)$ never exceeds 1.8% over the whole $\alpha \in [1, \infty)$ interval. It is moreover smaller than 0.2% for all values of $\alpha$ considered in the main text, save for the most heavily crosslinked simulated networks. As discuss in the text, these networks are not realistic from a biological standpoint, although they are interesting to consider from a conceptual standpoint.

Since $\beta$ is related to the dimensionless inverse of the network's volume $\alpha$ though Eq. (S33), the combination of Eq. (S33) and (S40) provides the stress-volume relation for undercoordinated branched networks and thus the analog of Eq. (S23). This relation is shown as $\tilde{\sigma}(\alpha)$ in Fig. S9(a) and provides the theoretical curves of Figs. 3(A) and (D) of the main text. The lower integration bound $\beta_0$ in Eq. (S40) plays the same role as the integration constant $\sigma_\infty$ in Eq. (S23a). It sets the equilibrium volume of the network in the absence of an external pressure, and is physically determined by the specific way in which the network was assembled, as discussed in Sec. S4.4.

The compressional stiffness of the network is given by

$$\tilde{K} = V \frac{\mathrm{d}\tilde{\sigma}}{\mathrm{d}V} = \frac{\beta g_n(\beta)}{\lambda_n(\beta)} \tag{S44}$$

which implies the asymptotic regimes

$$\tilde{K} = \begin{cases} \frac{4}{1+n}\beta^2 & \text{for } \beta \ll 1 \\ \beta^3 & \text{for } \beta \gg 1 \end{cases}. \tag{S45}$$

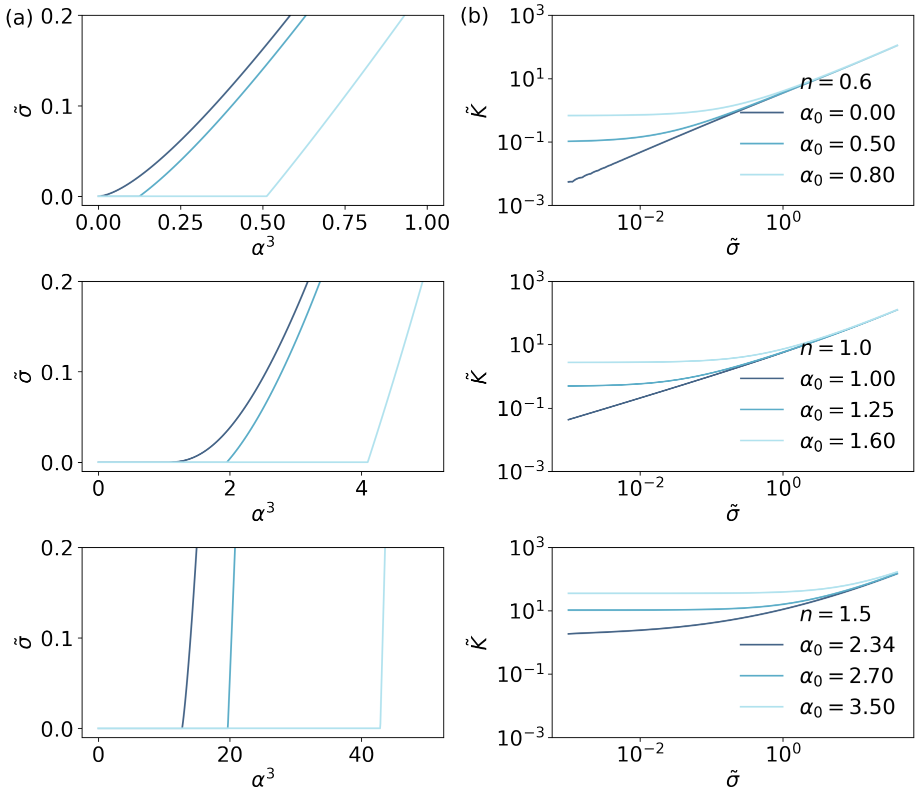


Figure S9: Constitutive relations predicted by the activated filament theory. (a) Dimensionless compressive stress as a function of the dimensionless inverse volume $\alpha$ after Eq. (S40). By comparison, in the original van Wyk theory of Eq. (S23) all curves of this panel would be straight lines for $\tilde{\sigma} > 0$. This behavior is recovered asymptotically at high compressions $\alpha \to \infty$, where the activation probability $p$ goes to one. In both the original and the activated filament theory, $\tilde{\sigma}$ is defined up to an integration constant. Equivalently, we may define the value $\alpha_0$ at which $\tilde{\sigma}$ crosses the origin. The values used here are shown in the legend of panel (b). Larger values of $\alpha_0$ denote more precompressed networks. The darkest curve in each subpanel shows the least possible amount of precompression $\alpha_0 = \alpha^*$, and reveal that $\tilde{\sigma}$ *vs.* $\alpha^3$ curve becomes rounded, *i.e.*, less steep, at low compression compared to the original van Wyk theory and consistent with the experimental and simulations data. The lighter, larger-$\alpha_0$ curves are shifted-down versions of this initial curve, and show that precompression gradually abolishes this rounding. (b) Dimensionless tangent elastic modulus as a function of dimensionless imposed compressive stress. For $n \leq 1$ and $\alpha_0 = \alpha^*$, the tangential modulus $\tilde{K}$ goes to zero for vanishing compression $\tilde{\sigma} \to 0$. Larger values of $n$ or $\alpha_0$ lead to the emergence of a finite elastic plateau given by computing $\beta_0$ from $\alpha_0$ with Eq. (S33) and inserting into Eq. (S46).

The undercoordinated counterpart of Eq. (S24) is thus obtained by inverting Eq. (S40) to extract the relationship $\beta(\tilde{\sigma})$ and inserting into Eq. (S44). The resulting $\tilde{K}(\tilde{\sigma})$ relationship is illustrated in Fig. S9(b) and provides the theoretical curves in Figs. 3(B) and (E) of the main text. In particular, substituting $\tilde{\sigma} = 0$ in Eq. (S40) yields $\beta = \beta_0$. By substituting this result into Eq. (S44), we find that the linear response modulus of the network is given by

$$\tilde{K}_0 = \tilde{K}(\tilde{\sigma} = 0) = \frac{\beta_0 g_n(\beta_0)}{\lambda_n(\beta_0)}. \tag{S46}$$

Therefore a non-vanishing value of $\beta_0$ is directly associated with the emergence of a finite linear-response modulus in the network.

### S4.4 Prestrain resulting from growth under stress

Here we derive the mechanical characteristics resulting from growth against an opposing compressive stress in our finite filament lengths formalism, a generalization of Eq. (S27). In this context, the counterpart of computing $\sigma_\infty$ is the determination of the constant $\beta_0$ introduced in Eq. (S40), which provides the value of the network's plateau modulus through Eq. (S46).

In this new context, the opposing stress $\sigma_g$ is shared between the activated filaments at the surface of the network. Their surface density is equal to $pN\ell/V$, implying a typical lateral distance $\sqrt{V/(pN\ell)}$ between two load-bearing filaments. As in Sec. S4.1, the typical deflection $y$ of a filament over the course of the growth process is of the order of this distance. Thus the load borne by a filament with $k$ contacts reads

$$f(k) = \frac{\kappa}{\zeta(k)^3} y \approx \frac{\kappa}{\zeta(k)^3}\sqrt{\frac{V}{pN\ell}}. \tag{S47}$$

We average this quantity over all load-bearing filaments and divide it by the specific area per load-bearing filament to recover the growth stress:

$$\sigma_g = \frac{N\ell}{V}\sum_{k=1+n}^{+\infty}\mathcal{P}(k)f(k) = \frac{\bar{\delta}\alpha}{\sqrt{\bar{\alpha}r\ell}}\frac{\kappa}{\ell^3}h_n(\beta), \tag{S48}$$

where $\bar{\delta}$ is a dimensionless coefficient of order one and where we have defined

$$\begin{aligned} h_n(\beta) &= \sum_{k=1+n}^{+\infty}\frac{\beta^{k-1/2}}{k!}(k+1-n)^3 e^{-\beta} \\ &= \left[\beta^{5/2} + 3(2-n)\beta^{3/2} + (7-9n+3n^2)\beta^{1/2} + (1-n)^3\beta^{-1/2}\right]\lambda_n(\beta) \\ &\quad + \left[\beta^{5/2} + (5-2n)\beta^{3/2} - \frac{(1-n)^3}{n}\beta^{1/2}\right]\mu_n(\beta). \end{aligned} \tag{S49}$$

Using the dimensionless units of Eq. (S37), defining the dimensionless stress

$$\tilde{\Sigma} = \frac{\bar{\delta}\sqrt{\bar{\alpha}}}{\bar{\gamma}}\sqrt{\frac{d}{\ell}} \tag{S50}$$

and using Eq. (S33), we find that the value of $\beta_0$ is the solution of the following equation:

$$\frac{\tilde{\sigma}_g}{\tilde{\Sigma}} = \frac{\beta_0 h_n(\beta_0)}{\lambda_n(\beta_0)}. \tag{S51}$$

Physically, for growth stress values smaller than the dimensional counterpart of $\tilde{\Sigma}$, namely $\Sigma = \bar{\gamma}\kappa/(\bar{\alpha}\ell^3 d)\tilde{\Sigma}$, the growing network is in the low-compression regime where only a fraction of its filaments are activated [$p < 1$ in Fig. S8(b)]. By contrast, for higher values it crosses over into the universal van Wyk regime where virtually all filaments are activated ($p \simeq 1$). In the main text, we solve Eq. (S51) to obtain the value of $\beta_0$ as a function of the growth pressure in each curve of Fig. 3(a-f). While doing so we use $\Sigma$ as a global adjustable parameter whose value is the same for all curves. While Eq. (S51) is transcendental and must thus be solved numerically in general, it displays two analytically tractable asymptotic regimes:

$$\frac{\tilde{\sigma}_g}{\tilde{\Sigma}} = \frac{\sigma_g}{\Sigma} = \begin{cases} \frac{8}{1+n}\beta_0^{3/2} & \text{for } \tilde{\sigma}_g/\tilde{\Sigma} \ll 1 \\ \beta_0^{7/2} & \text{for } \tilde{\sigma}_g/\tilde{\Sigma} \gg 1 \end{cases}. \tag{S52}$$

The $\tilde{\sigma}_g/\tilde{\Sigma} \gg 1$ regime, which describes strongly compressed networks, is more likely to be reached when $\tilde{\Sigma}$ is small. This is the case when the length $\ell$ of the filaments is very large [Eq. (S50)], which

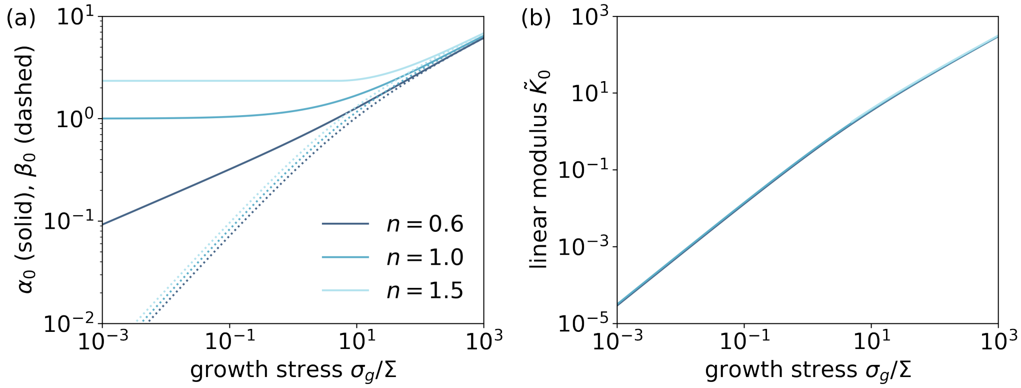


Figure S10: Effect of a growth stress on a branched network. (a) Number of contacts $\alpha_0$ and of activated contacts $\beta_0$ per filament that are trapped in the network as a result of the stressed growth process and therefore subsequently subsist even in the absence of an externally applied stress. These curves are obtained by solving Eq. (S51) and applying Eq. (S33) to obtain $\alpha_0$. In $n \geq 1$ systems with a first-order percolation transition, even the most minute growth stress forces the system to sit just above the percolation transition. As a result, for $\sigma_g \to 0$ the number of trapped contacts $\alpha_0$ goes to the critical number of contacts $\alpha^*$ defined in Sec. S4.2. (b) Linear modulus of the network as a function of growth stress obtained by applying Eq. (S46) to the three sets of curves studied in the first panel. The three different values of $n$ are almost indistinguishable. This can be understood from the weak dependence of $\tilde{K}_0$ on $n$ in the low growth stress asymptotic regime of Eq. (S53), as well as from the requirement that the influence of $n$ on the network's mechanics must disappear at large stresses.

constitutes the limit where we expect to recover the asymptotic behavior of Eq. (S26). To show that this is indeed the case, we first note that for strong compression $\beta = \alpha \approx \ell/\zeta$. The scaling of Eq. (S26) can then be recovered by inserting this result into the second regime of Eq. (S52). In practice, the data presented in Fig. 3 of the main text is equally well fitted by using Eq. (S51) [with the stress $\Sigma$ as a fitting parameter] or the asymptotic formula of Eq. (S26) (using the multiplicative prefactor as a fitting parameter). This indicates that the simpler, strong compression theory of Sec. S4.1 is a good description of the accumulation of contacts during stressed growth in our experiments. We display the full behavior of the solution of Eq. (S51) in Fig. S10(a), both in terms of the number of trapped activated contacts $\beta_0$ and in terms of the number of total contact $\alpha_0$.

Combined with Eqs. (S45-S46), Eq. (S52) implies that the linear modulus induced by a growth stress is an increasing function of that growth stress with asymptotic regimes

$$\tilde{K}_0\left(\frac{\sigma_g}{\Sigma}\right) = \begin{cases} (1+n)^{1/3}(\sigma_g/\Sigma)^{4/3} & \text{for } \tilde{\sigma}_g/\tilde{\Sigma} \ll 1 \\ (\sigma_g/\Sigma)^{6/7} & \text{for } \tilde{\sigma}_g/\tilde{\Sigma} \gg 1 \end{cases}, \tag{S53}$$

where the latter asymptotic regime recapitulates the result of Eq. (S27).

## S4.5 Mechanical response in the presence of crosslinkers

To model the effect of crosslinkers in our branched, weakly coordinated networks, we assume that their effect is to force permanent contacts between pairs of filaments. Denoting by $x$ the average number of crosslinker-induced contacts per filament, the total average number of contacts per filament is thus $x + \alpha$, where the number $\alpha$ of transient contacts is still given by Eq. (S28). The mean number of active contacts then reads $\beta = (\alpha + x)p$, and the self-consistency Eq. (S33) is replaced by

$$\frac{\beta}{\alpha + x} = \lambda_n(\beta). \tag{S54}$$

All other results derived in the absence of crosslinkers then proceed from there by replacing $\alpha$ by $\alpha+x$. The values of $\beta_0$ used in the analytical curves of Fig. 4(A-F) of the main text are thus obtained by fixing $\alpha$ to the values of $\alpha_0$ determined in determined in Fig. 3(A-F) of the main text in Eq. (S54) and solving it for different values of $x$. The theoretical curves of Figs. 4(A-B) and (D-E) are further obtained by solving Eq. (S54) for $\beta$ and inserting the result into Eqs. (S40) and (S44).

## S4.6 Branch length estimates and consistency checks based on fitting parameters

The fits of our theoretical model reported in Fig. 3 the main text yield numerical values for several parameters pertaining to our experimental and simulated networks. The first of these parameters is the per-filament number $n$ of missing contacts to isostaticity. The second is the stress scaling factor involved in the adimensionalization of Eq. (S37), which we write as

$$\sigma_{\text{typ}} = \frac{\bar{\gamma}}{\bar{\alpha}} \frac{\kappa}{\ell^3 d}. \tag{S55}$$

The third parameter depends on the dataset considered. In the case of the numerical simulations it reads [Eq. (S28)]

$$\alpha_0 = \alpha(\gamma_p = 0, \gamma = 0) = \bar{\alpha} \frac{N\ell^2 d}{V}, \tag{S56}$$

where $N/V$ is to be understood as the density of filaments in the non-prestrained ($\gamma_p = 0$), undeformed ($\gamma = 0 \Leftrightarrow \sigma = 0$) system. In the case of the experimental data, the third parameter is instead [Eq. (S50)]

$$\Sigma = \frac{\bar{\delta}}{\bar{\alpha}^{1/2}} \frac{\kappa}{\ell^{7/2} d^{1/2}}. \tag{S57}$$

Unlike the parameter $n$, the parameters listed in Eqs. (S55-S57) combine several of the model's microscopic parameters. Here we discuss them to extract more physically transparent information from them and perform consistency checks to reveal whether our theoretical model is indeed a good description of the experimental and simulated data.

Our fitting procedure applied to our simulations data yields $\sigma_{\text{typ}} = 2.62 \times 10^{-3}$ and $\alpha_0 = 1.11$ in simulations units. We recall that our simulations units are chose to match the values of the bending modulus $\kappa = 4 \times 10^{-26}\,\text{J} \cdot \text{m}$ and mesh size $\xi = 40\,\text{nm}$ typical of branched actin networks. Finally, the branching process described in Sec. S3.1 implies that $\ell = 2d/b \approx 2\xi/\sqrt{b}$, and we use a branching rate $b = 0.1$ in all simulations presented in the main text. Combining these three pieces of information with Eqs. (S55) and (S56) yields the following numerical equations in physical units:

$$\sqrt{b}\ell/2 = 40\,\text{nm} \tag{S58a}$$

$$\frac{\bar{\gamma}}{\bar{\alpha}} \frac{\kappa}{\ell^3 d} = 256\,\text{Pa} \tag{S58b}$$

$$\bar{\alpha} \frac{N\ell^2 d}{V} = 1.11, \tag{S58c}$$

where we compute the average initial filament concentration resulting from the network preparation protocol of Sec. S3.1 as $N/V = 0.00776 d^{-3}$ from geometrical considerations. We recall that in Eqs. (S58), the dimensionless constants $\bar{\alpha}$ and $\bar{\gamma}$ are undetermined geometrical prefactors of order one. A first possible approach would be to set these constants to one, and view the three equations of Eqs. (S58) as three independent readouts on the order of magnitude of the filament length $\ell$. We could then check the consistency of our theoretical model by asking whether the $\ell$-values derived from each of the three equations are compatible. Equivalently, we can consider Eqs. (S58) as a system of equations for the three unknowns $\ell$, $\bar{\alpha}$ and $\bar{\gamma}$, solve it, and check that the values of the two dimensionless

constants are of order one as they should be. Doing so yields

$$\ell \simeq 253\,\text{nm} \tag{S59a}$$
$$\bar{\alpha} \simeq 0.358 \tag{S59b}$$
$$\bar{\gamma} \simeq 0.469, \tag{S59c}$$

which is the basis of the numerical values reported in the main text. The values of $\bar{\alpha}$ and $\bar{\gamma}$ confirm that our theoretical descriptions of the morphology and the mechanics of our simulated network are consistent. Note that the geometrical factors $\bar{\alpha}$ and $\bar{\gamma}$ characterize not only the initial state of the network, but also the complex random geometry of its compressed state. They are therefore difficult to accurately compute from first principles, and we do not attempt to do so.

Our fits to our experimental results yield $\sigma_{\text{typ}} = 794\,\text{Pa}$ and $\Sigma = 17.3\,\text{Pa}$. In contrast with the simulations case, we do not have any direct characterization of the branch length in our networks. Using Eqs. (S55) and (S57) and the values of $\bar{\alpha}$ and $\bar{\gamma}$ derived in Eq. (S59), we can thus recast the values of our two fitting parameters as two equations

$$\frac{\kappa}{\ell^3 d} = 606\,\text{Pa} \tag{S60a}$$
$$\bar{\delta}\frac{\kappa}{\ell^{7/2} d^{1/2}} = 10.4\,\text{Pa}, \tag{S60b}$$

where the diameter $d = 8\,\text{nm}$ of actin filaments is well characterized. Similar to our strategy in the previous paragraph, we solve these equations for $\ell$ and the dimensionless constant $\bar{\delta}$ and find

$$\ell \simeq 202\,\text{nm} \tag{S61a}$$
$$\bar{\delta} \simeq 0.0859, \tag{S61b}$$

which is the basis of the numerical values reported in the main text. Again, we find that our geometrical parameter (here $\bar{\delta}$) is of order one, indicating that our theoretical model gives a consistent description of our experimental branched network.

## References


[1] James C Maxwell. On the calculation of the equilibrium and stiffness of frames. *Philos. Mag.*, 27:294–299, 1864.

[2] C R Calladine. Buckminster Fuller's "tensegrity" structures and Clerk Maxwell's rules for the construction of stiff frames. *Int. J. Solids Structures*, 14(2):161–172, 1978.

[3] Chase P Broedersz, Xiaoming Mao, Tom C Lubensky, and Frederick C MacKintosh. Criticality and isostaticity in fibre networks. *Nat. Phys.*, 7:983–988, December 2011.

[4] C P Broedersz and F C MacKintosh. Modeling semiflexible polymer networks. *Rev. Mod. Phys.*, 86:995–1036, July-September 2014.

[5] Thomas Pujol, Olivia du Roure, Marc Fermigier, and Julien Heuvingh. Impact of branching on the elasticity of actin networks. *Proc. Natl. Acad. Sci. U.S.A.*, 109(26):10364–10369, June 2012.

[6] Pierre Bauër, Joseph Tavacoli, Thomas Pujol, Jessica Planade, Julien Heuvingh, and Olivia du Roure. A new method to measure mechanics and dynamic assembly of branched actin networks. *Sci. Rep.*, 7(1):15688, Nov 2017.

[7] Joe W. Tavacoli, Pierre Bauër, Marc Fermigier, Denis Bartolo, Julien Heuvingh, and Olivia du Roure. The fabrication and directed self-assembly of micron-sized superparamagnetic non-spherical particles. *Soft Matter*, 9:9103–9110, 2013.

[8] T P Loisel, Rajaa Boujemaa-Paterski, D Pantaloni, and Marie-France Carlier. Reconstitution of actin-based motility of Listeria and Shigella using pure proteins. *Nature*, 401(6753):613–6, oct 1999.

[9] Anne Bernheim-Groswasser, Sebastian Wiesner, Roy M Golsteyn, Marie-France Carlier, and Cécile Sykes. The dynamics of actin-based motility depend on surface parameters. *Nature*, 417(6886):308–311, 2002.

[10] A "primer"-based mechanism underlies branched actin filament network formation and motility. *Current Biology*, 20(5):423–428, mar 2010.

[11] Belbahri Reda, Michelot Alphée, Heuvingh Julien, and du Roure Olivia. Non-linear elastic properties of actin patches to partially rescue yeast endocytosis efficiency in the absence of the cross-linker sac6. *Soft Matter*, 18:1479–1488, 2022.

[12] Gary S Grest and Kurt Kremer. Molecular dynamics simulation for polymers in the presence of a heat bath. *Physical Review A*, 33(5):3628, 1986.

[13] Kurt Kremer and Gary S Grest. Dynamics of entangled linear polymer melts: A molecular-dynamics simulation. *The Journal of Chemical Physics*, 92(8):5057–5086, 1990.

[14] John D Weeks, David Chandler, and Hans C Andersen. Role of repulsive forces in determining the equilibrium structure of simple liquids. *The Journal of chemical physics*, 54(12):5237–5247, 1971.

[15] A Allard, Mehdi Bouzid, T Betz, C Simon, M Abou-Ghali, J Lemière, F Valentino, J Manzi, F Brochard-Wyart, K Guevorkian, et al. Actin modulates shape and mechanics of tubular membranes. *Science advances*, 6(17):eaaz3050, 2020.

[16] Aidan P Thompson, H Metin Aktulga, Richard Berger, Dan S Bolintineanu, W Michael Brown, Paul S Crozier, Pieter J in't Veld, Axel Kohlmeyer, Stan G Moore, Trung Dac Nguyen, et al. Lammps-a flexible simulation tool for particle-based materials modeling at the atomic, meso, and continuum scales. *Computer Physics Communications*, 271:108171, 2022.

[17] Aidan P Thompson, Steven J Plimpton, and William Mattson. General formulation of pressure and stress tensor for arbitrary many-body interaction potentials under periodic boundary conditions. *The Journal of chemical physics*, 131(15), 2009.

[18] C. M. van Wyk. 20—note on the compressibility of wool. *Journal of the Textile Institute Transactions*, 37(12):T285–T292, 1946.

[19] Staffan Toll. Packing mechanics of fiber reinforcements. *Polymer Engineering and Science*, 38(8):1337, August 1998.
